# Supplementary material for: Effects of capturing a wide-orbit planet on planetary systems: system stability and Habitable Zone bombardment rates
Source: arXiv:2010.15448 source file (2020-10-29)
Supplement: Supplementary file 1 [file old_appendix.tex]

\begin{figure}
    \centering
    \includegraphics[width=\columnwidth]{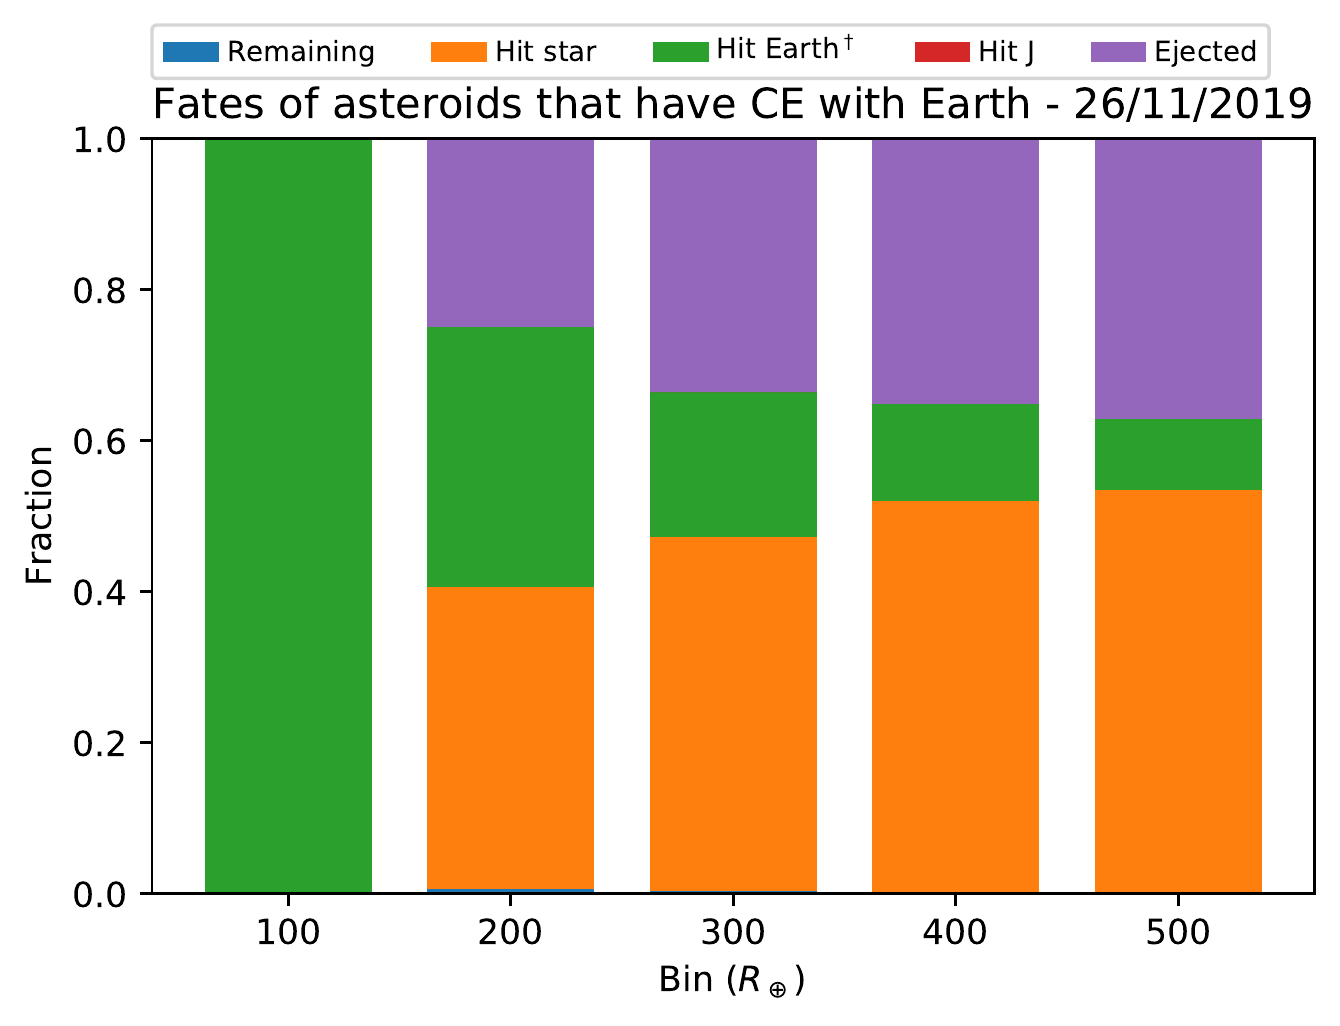}
    \caption{The final outcome of asteroids that have a close encounter with the Earth in the ck1.4 run, where each bin holds all asteroids that have a close encounter within the number given on the x-axis.}
    \label{fig:post_E_CE}
\end{figure}
\textcolor{green}{10) Given Earth CE, what happens after?}\\
\textit{Figure~\ref{fig:post_E_CE} shows the final outcome for all the asteroids that have a close encounter with the Earth, binned by how close they get. Out of the 90\% that do not end up hitting the Earth we see a fairly even split between hitting the star and being ejected as the final outcome.}
\section{Figures}
\begin{figure}
    \centering
    \includegraphics[width=\columnwidth]{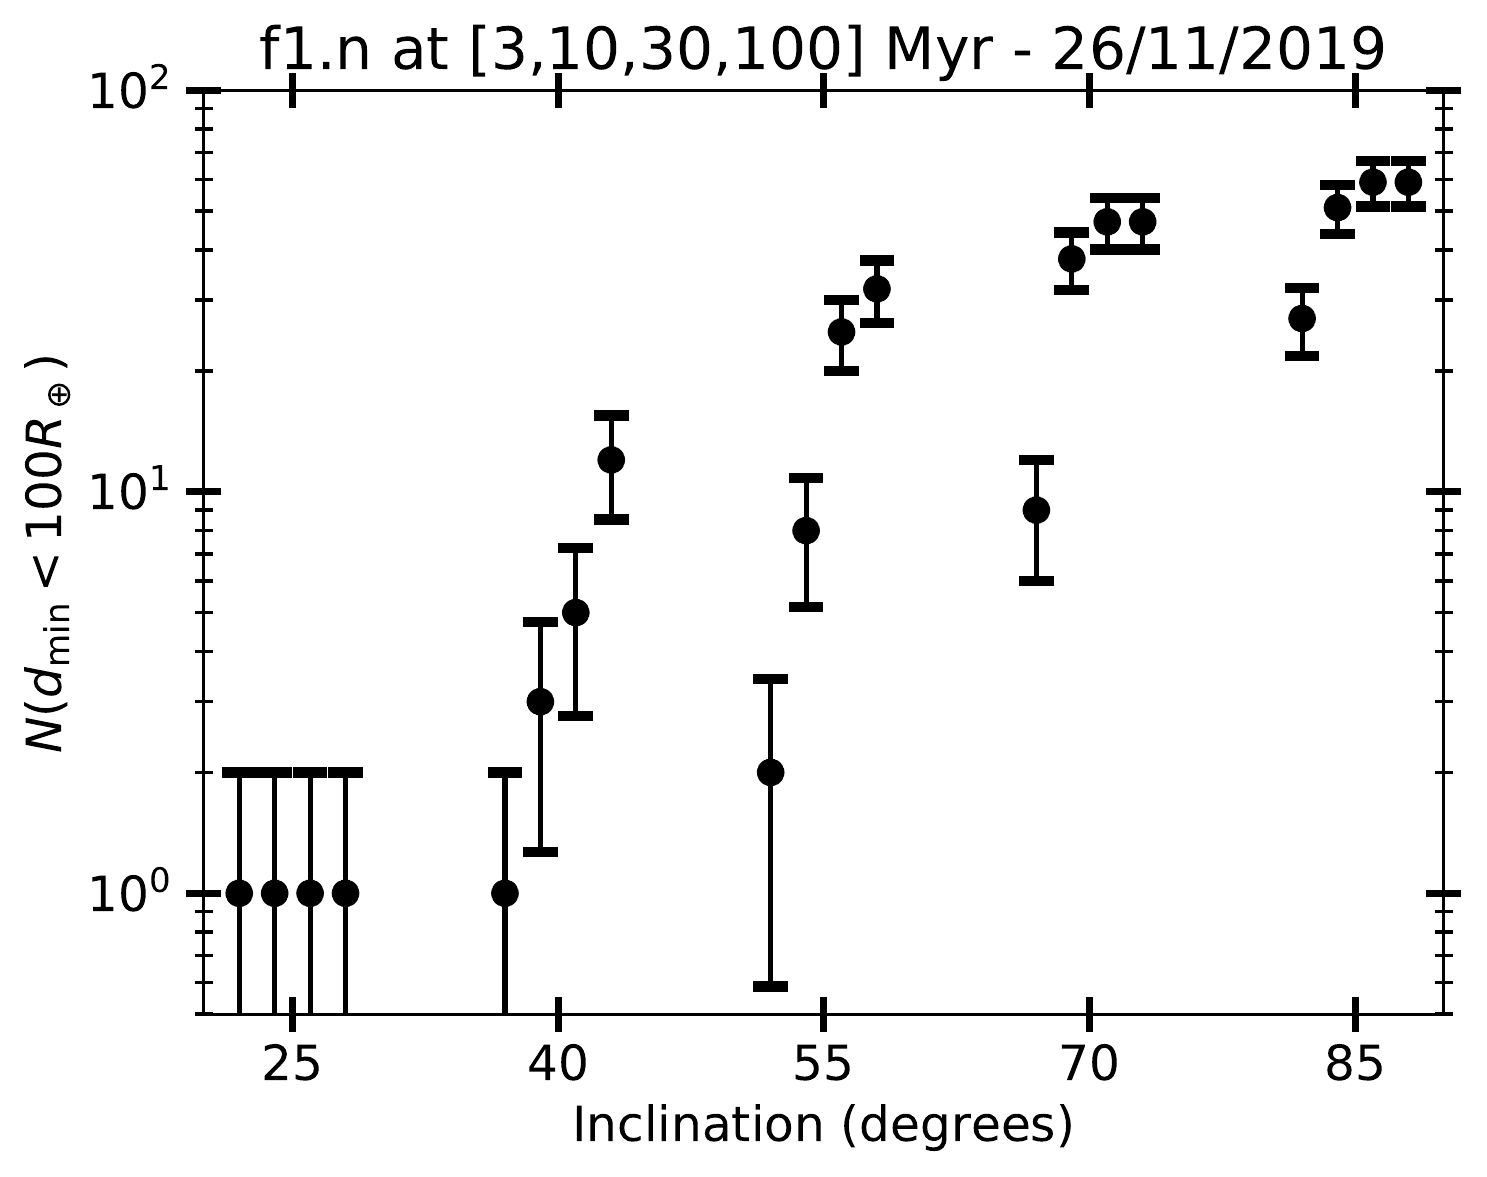}
    \caption{The number of hits for the f1.n runs at four different times = [3, 10, 30, 100] Myr.}
    \label{fig:hits_v_t}
\end{figure}
\begin{figure}
    \centering
    \includegraphics[width=\columnwidth]{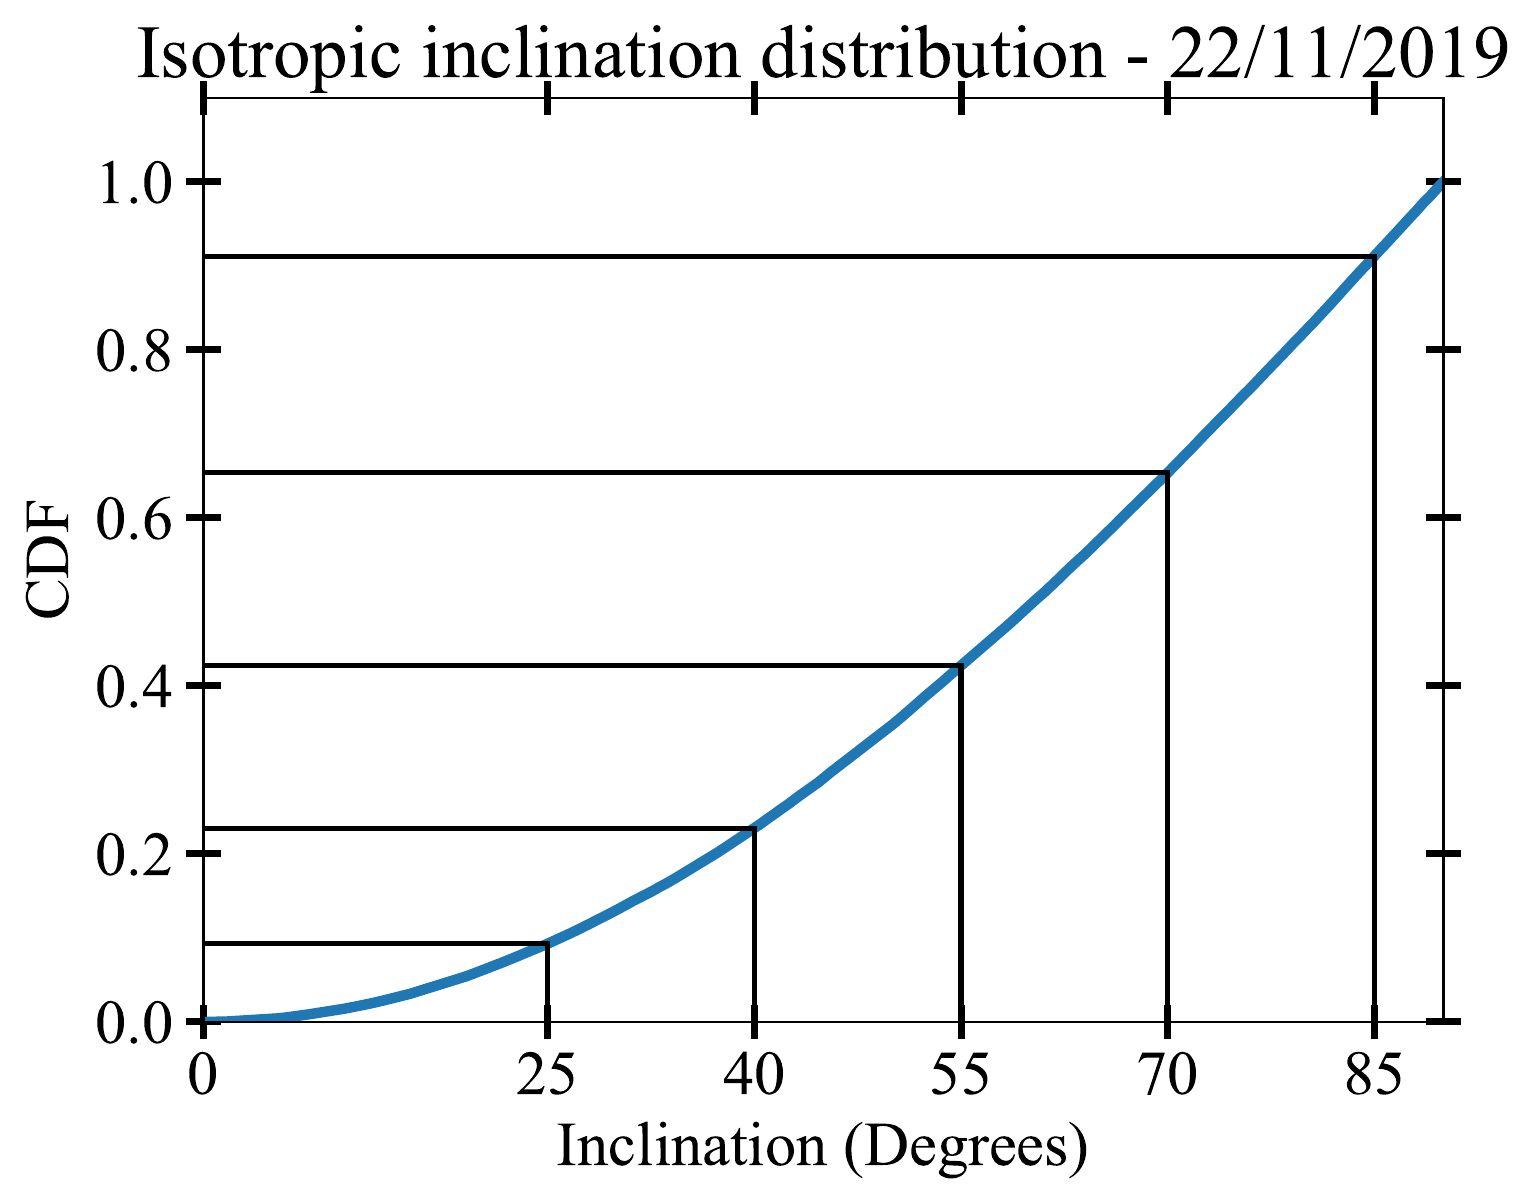}
    \caption{The inclination distribution of isotropically captured planets.}
    \label{fig:isotropic}
\end{figure}
\begin{figure}
    \centering
\includegraphics[width=\columnwidth]{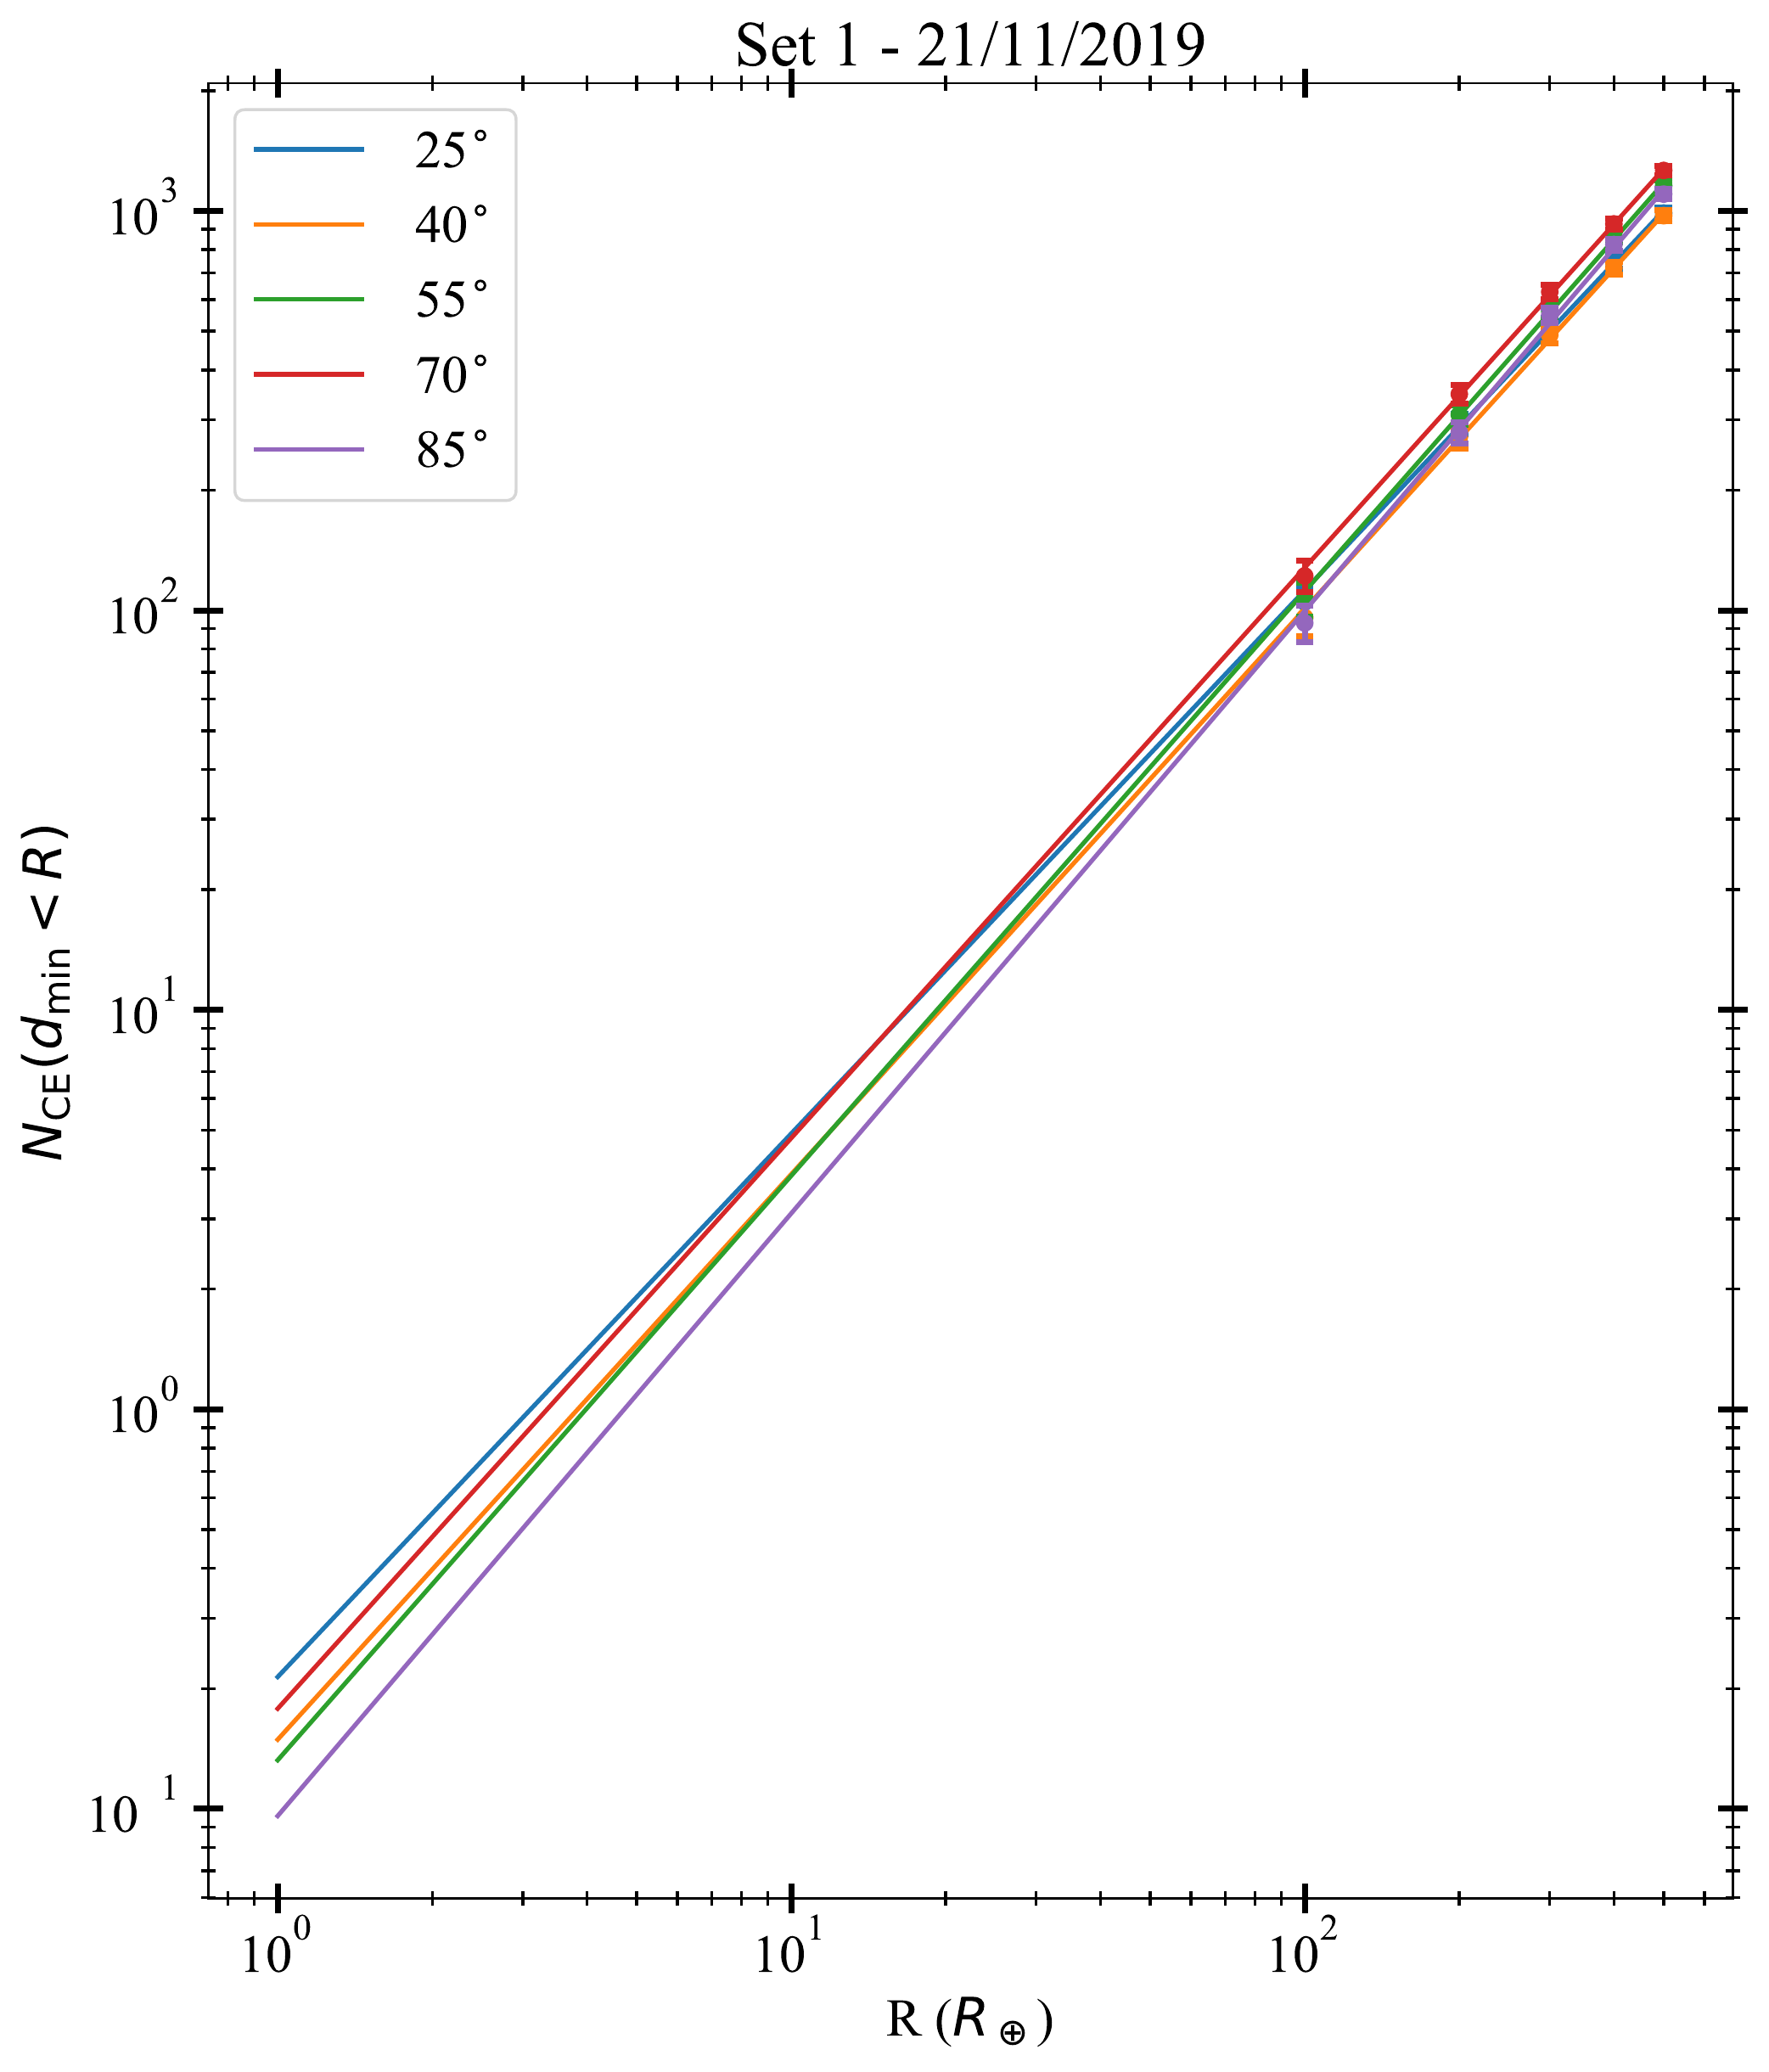}
    \caption{log-log version of~\ref{fig:fit}.}
    \label{fig:loglog}
\end{figure}
\begin{figure}
    \centering
    \includegraphics[width=\columnwidth]{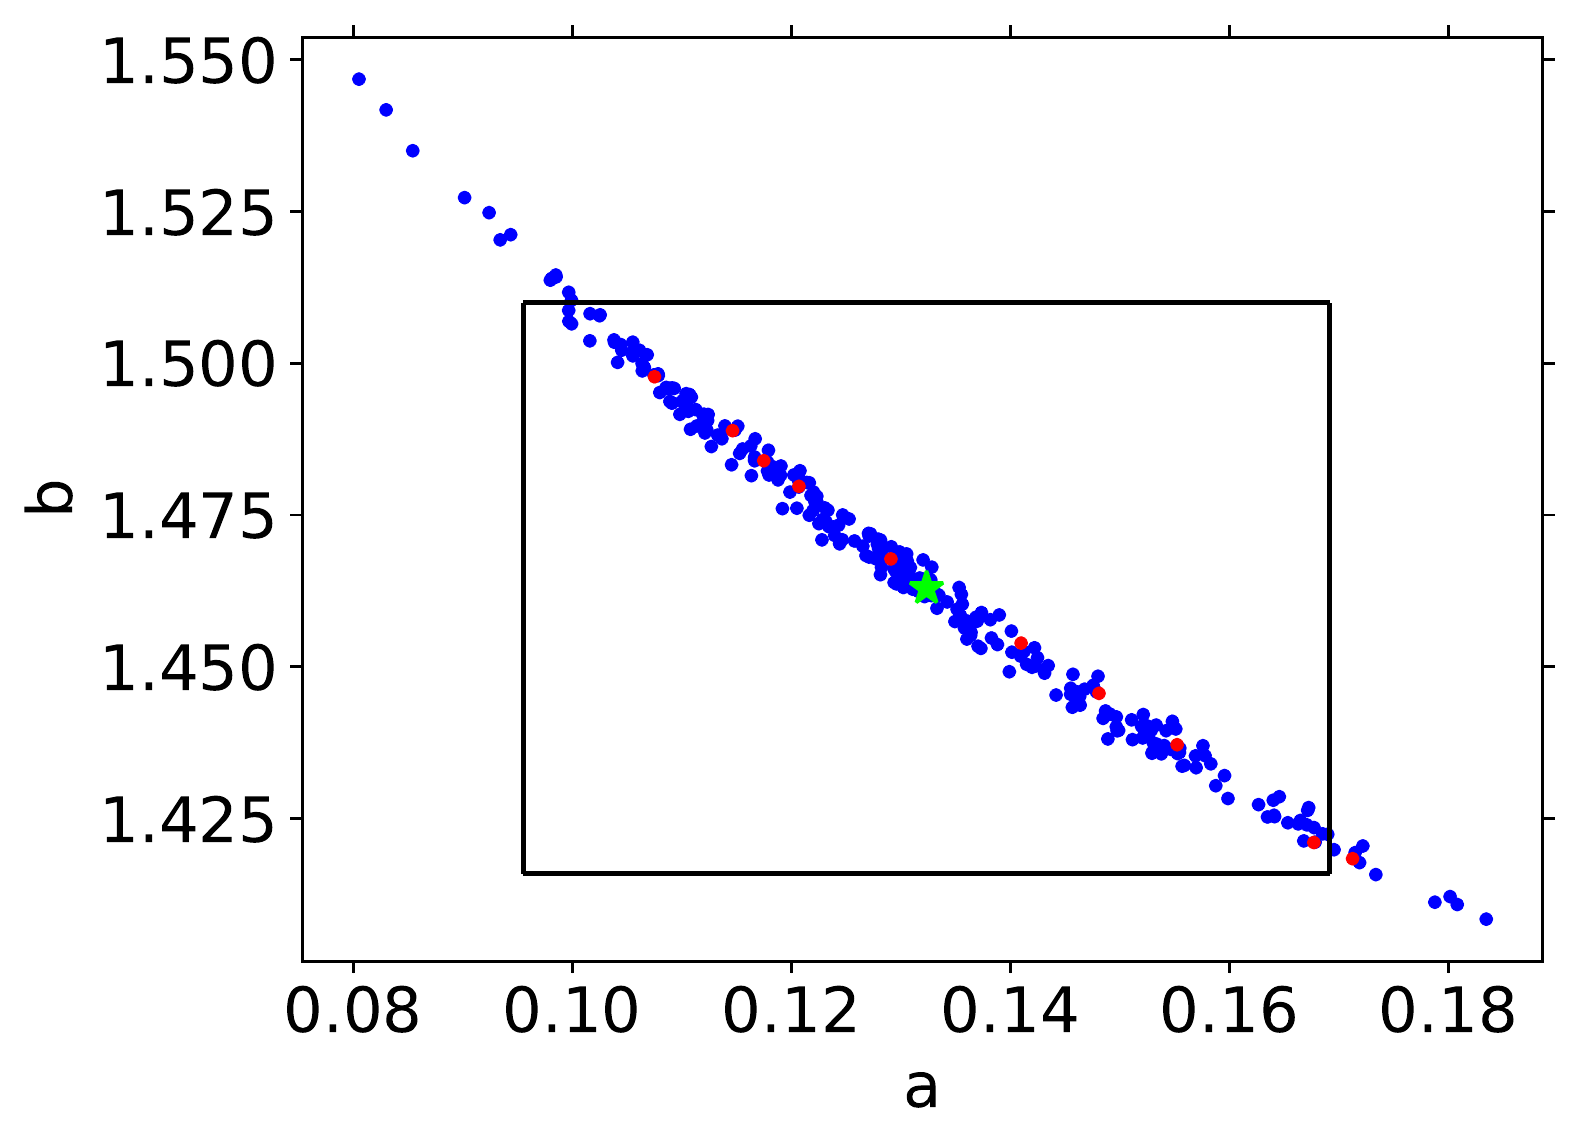}
    \caption{Covariance of the a and b fit to the different ck lines and shown in table~\ref{tab:ab}.}
    \label{fig:covariance}
\end{figure}
\begin{figure}
    \centering
    \includegraphics[width=\columnwidth]{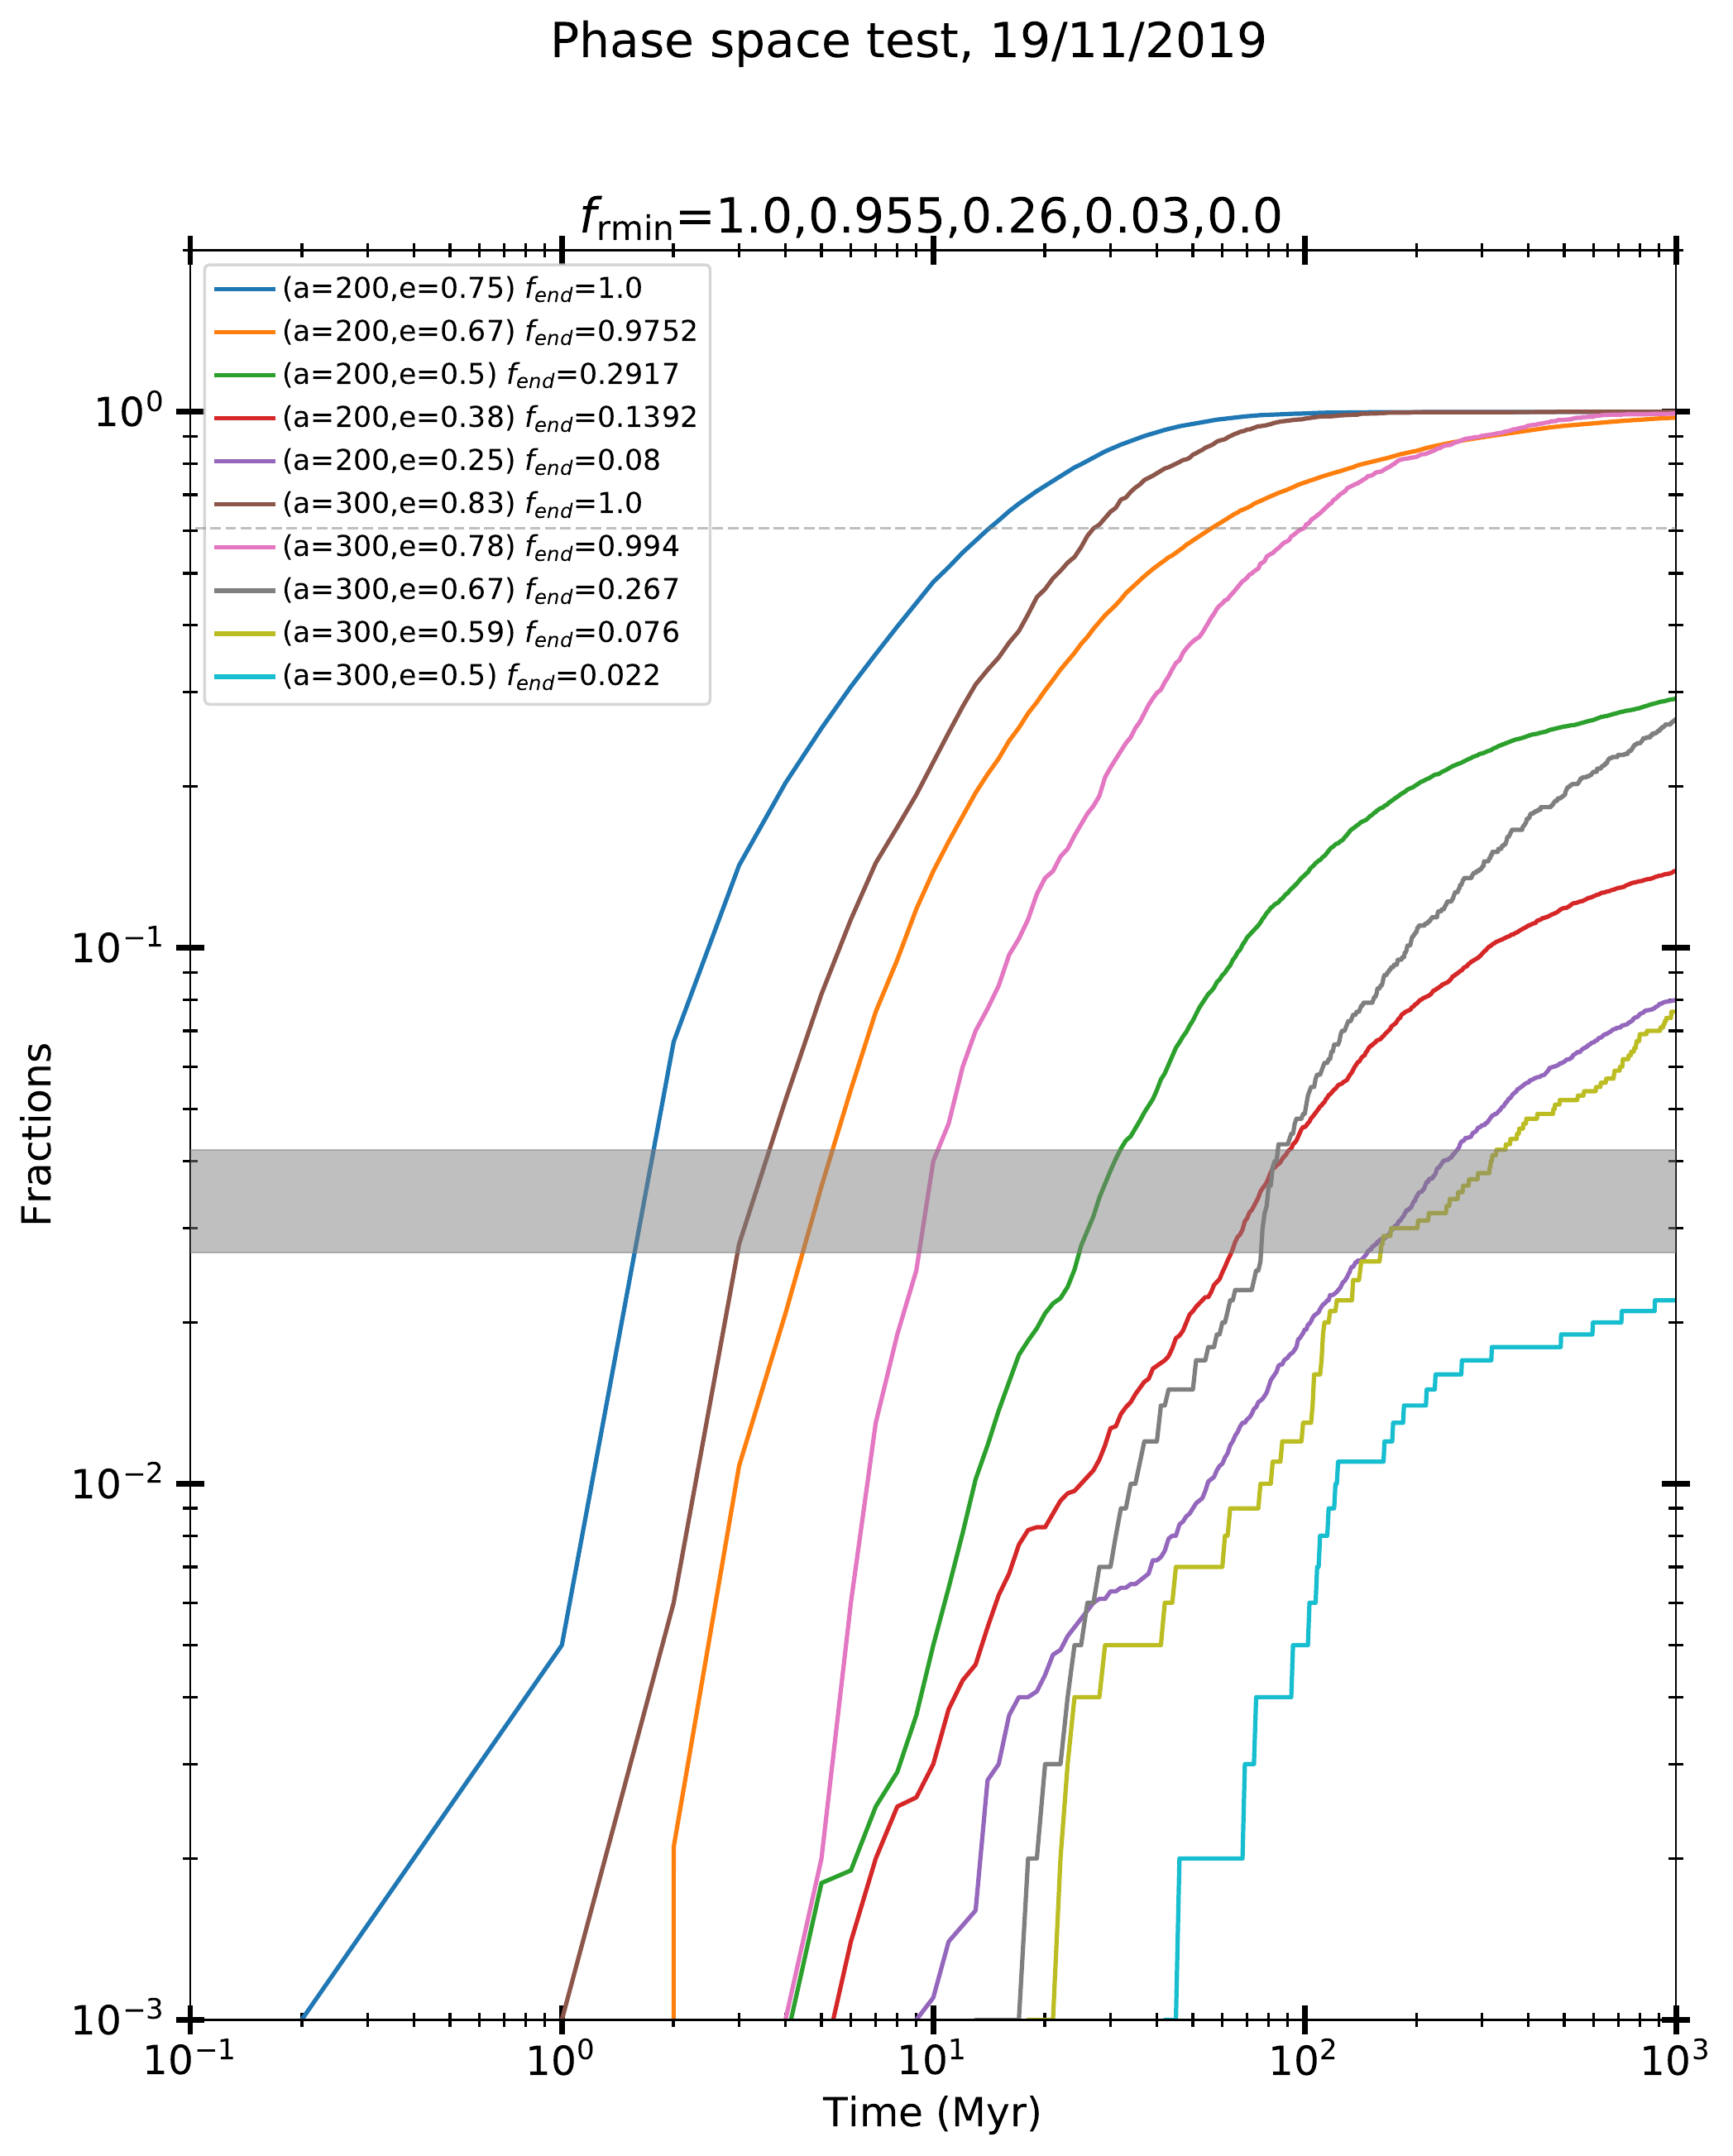}
    \caption{CDFs of remaining particles for 1Gyr fne simulations done with $I_c=40$ at locations marked in figure~\ref{fig:regimes}.}
    \label{fig:my_label}
\end{figure}
\begin{figure}
    \centering
    \includegraphics[width=\columnwidth]{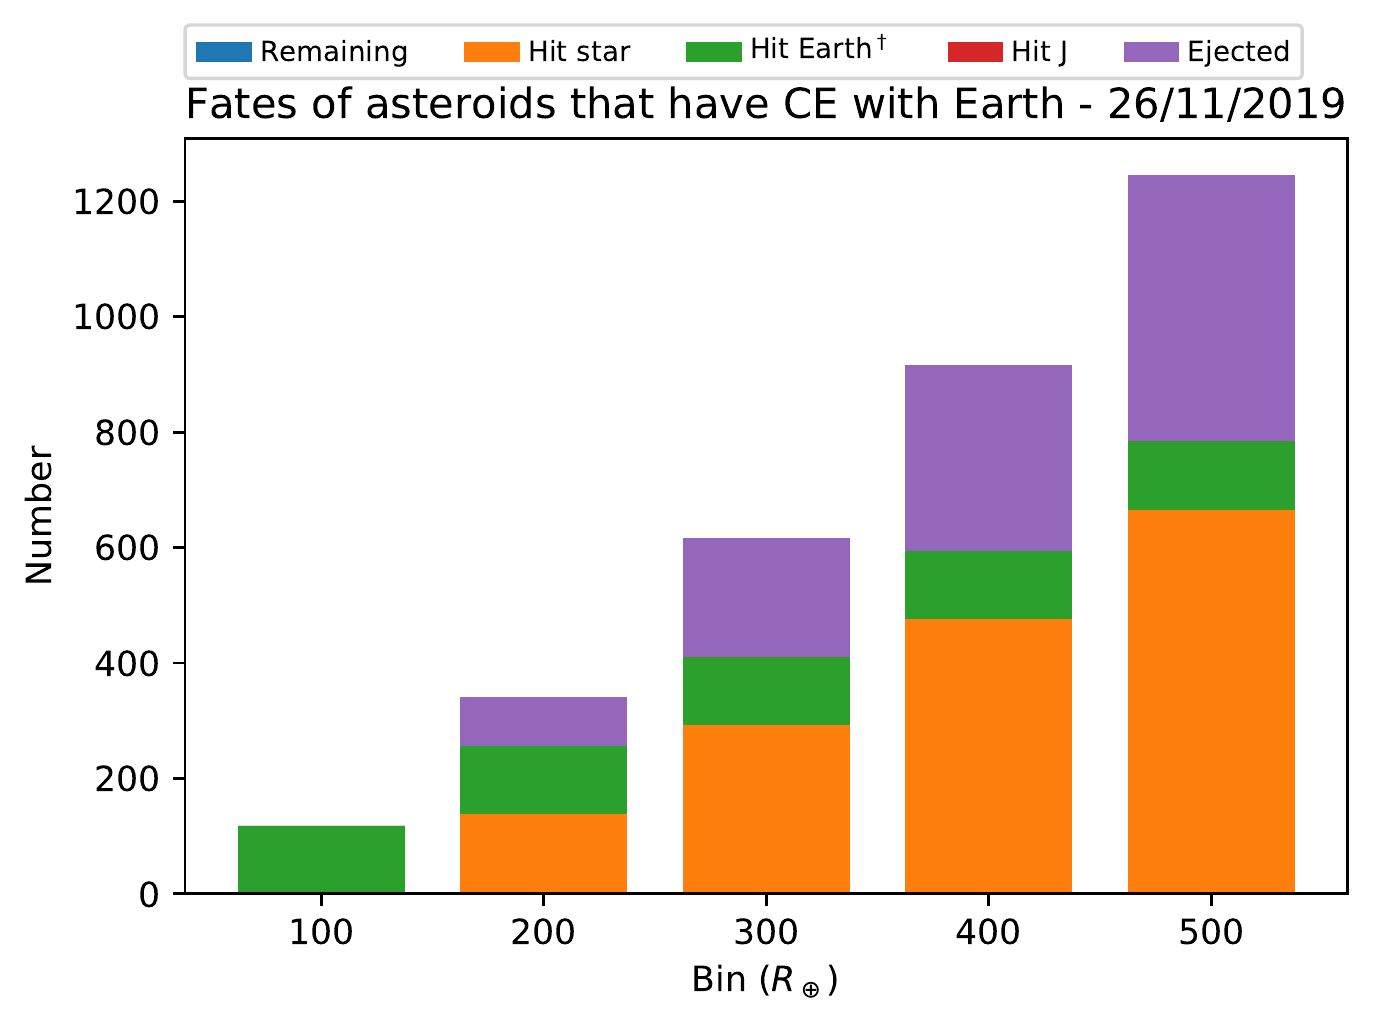}
    \caption{Numbers rather than fractions for fates of asteroids that have a close encounter with Earth.}
    \label{fig:bar_numbers}
\end{figure}
\begin{figure}
    \centering
    \includegraphics[width=\columnwidth]{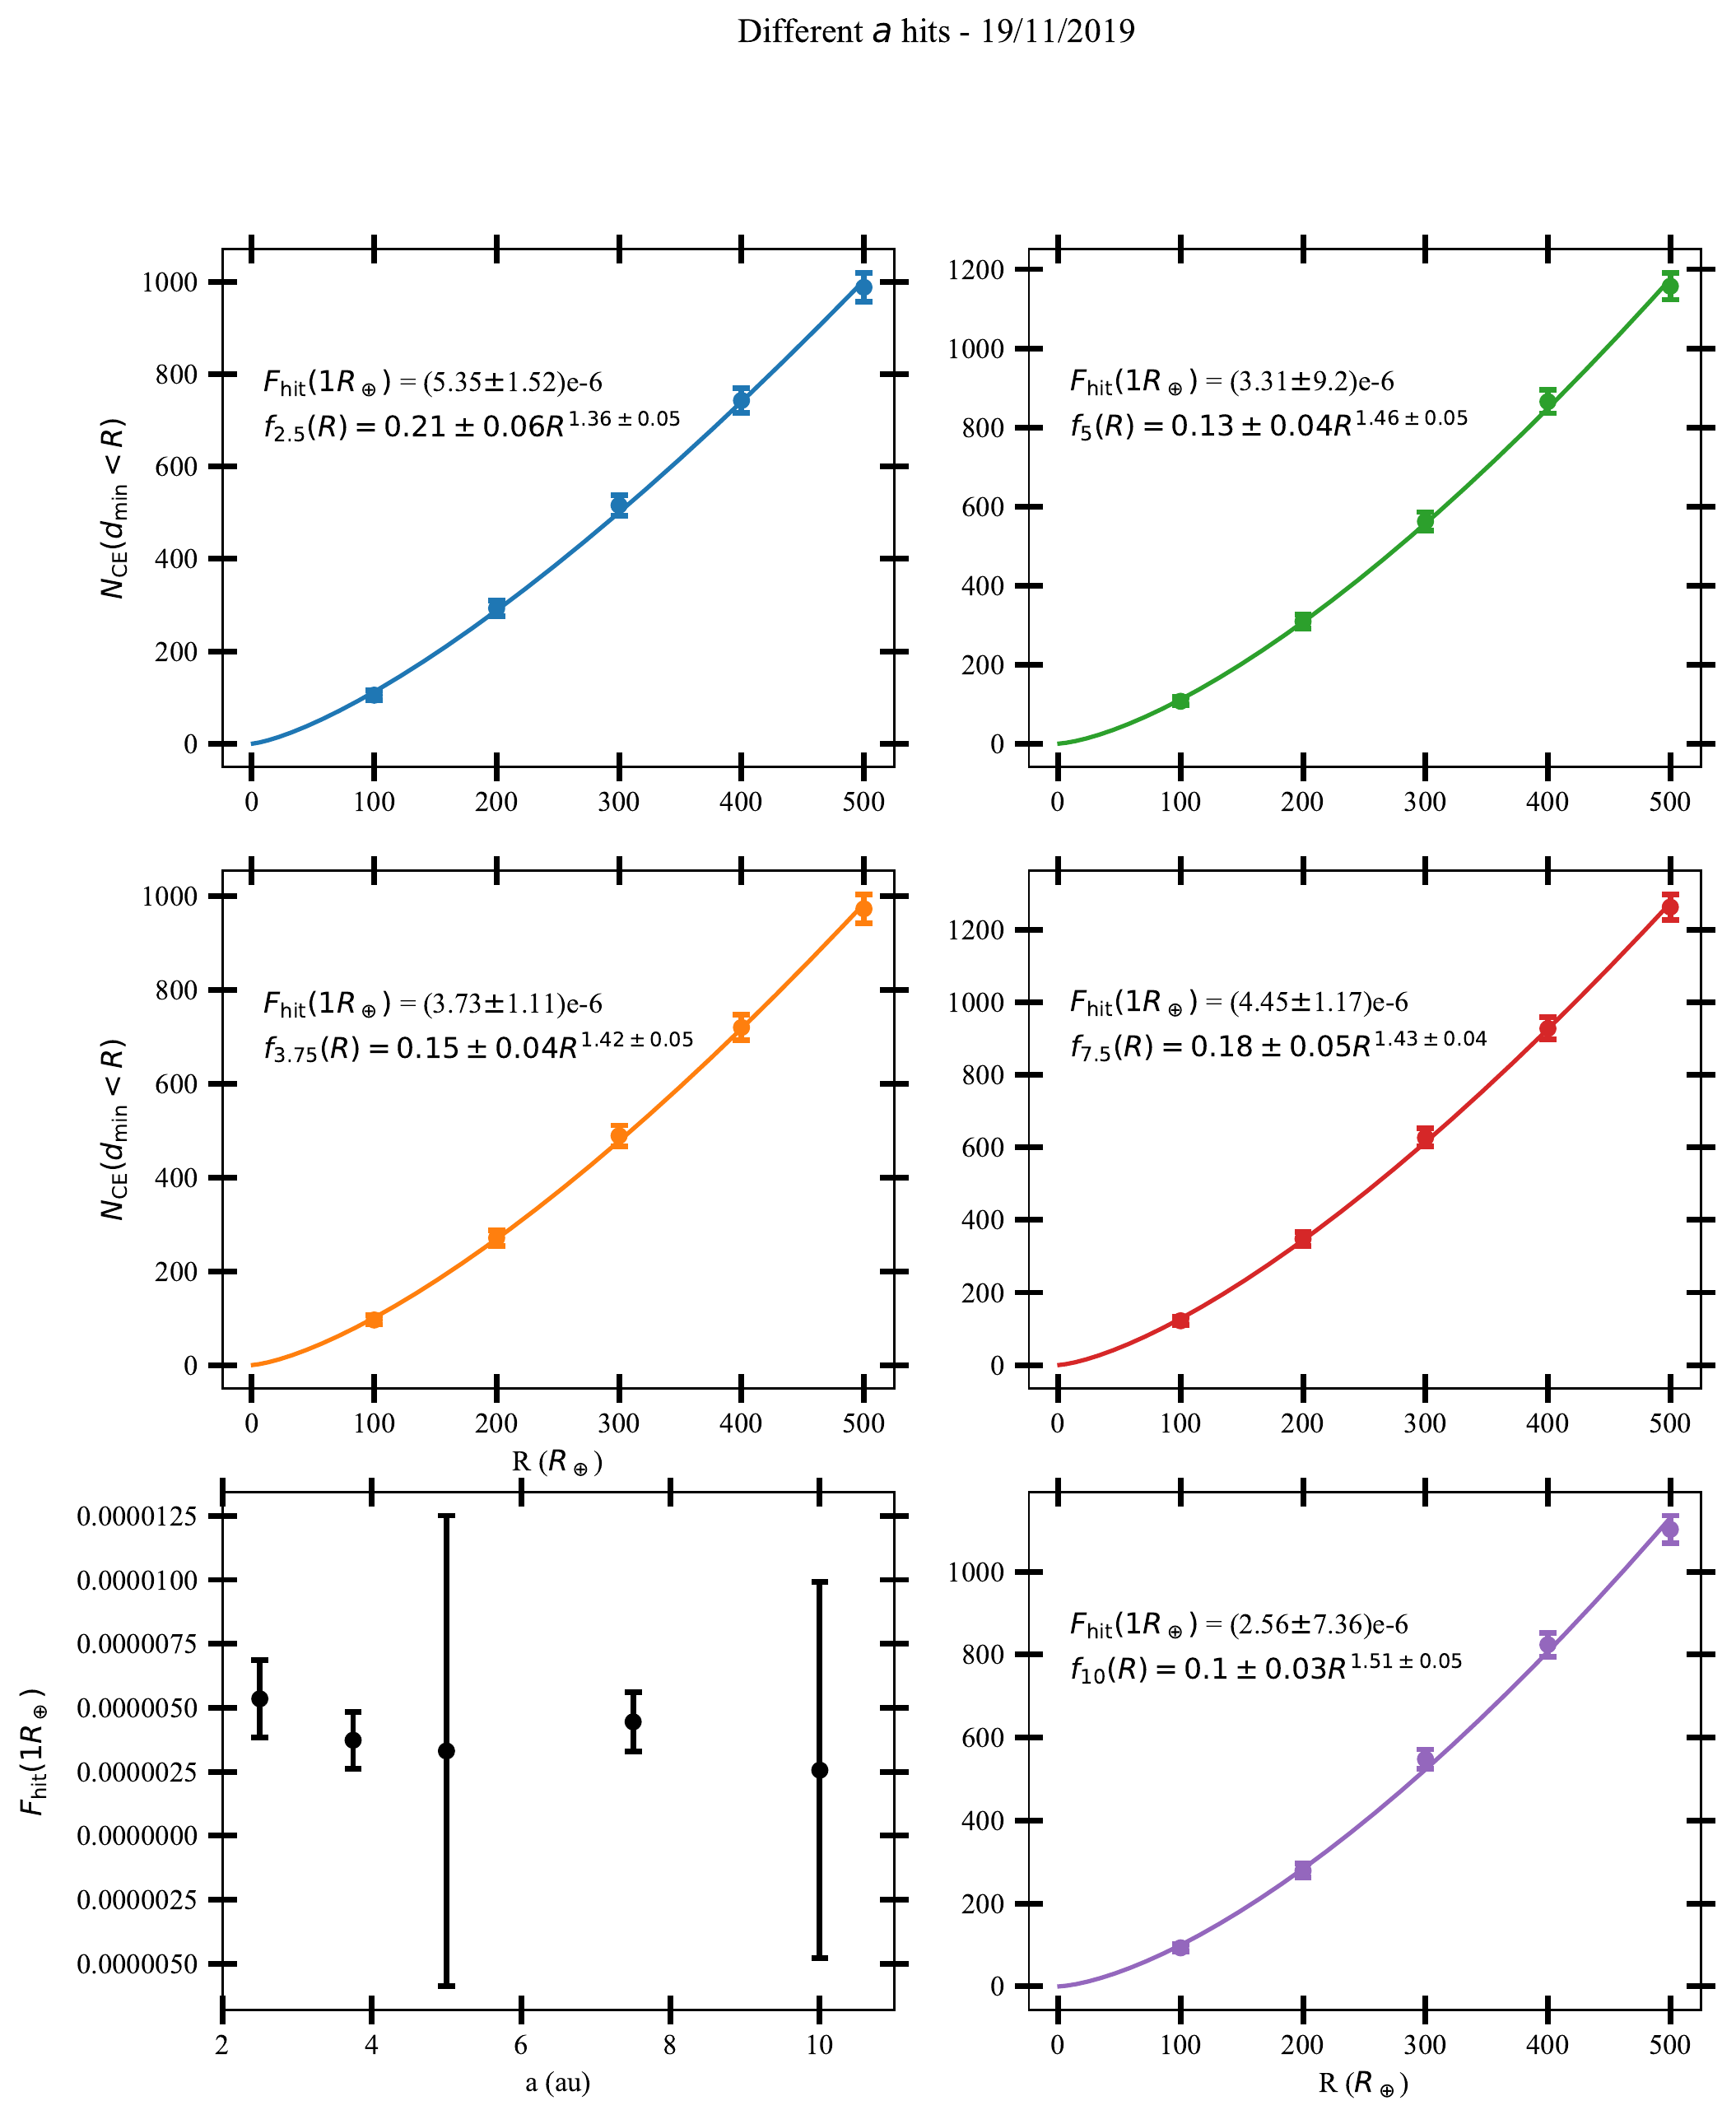}
    \caption{The hit rate on Earth for a set of ck runs for $I_c=70$ degrees with changing $a_J$.}
    \label{fig:a_E_hits}
\end{figure}
\begin{figure}
    \centering
    \includegraphics[width=\columnwidth]{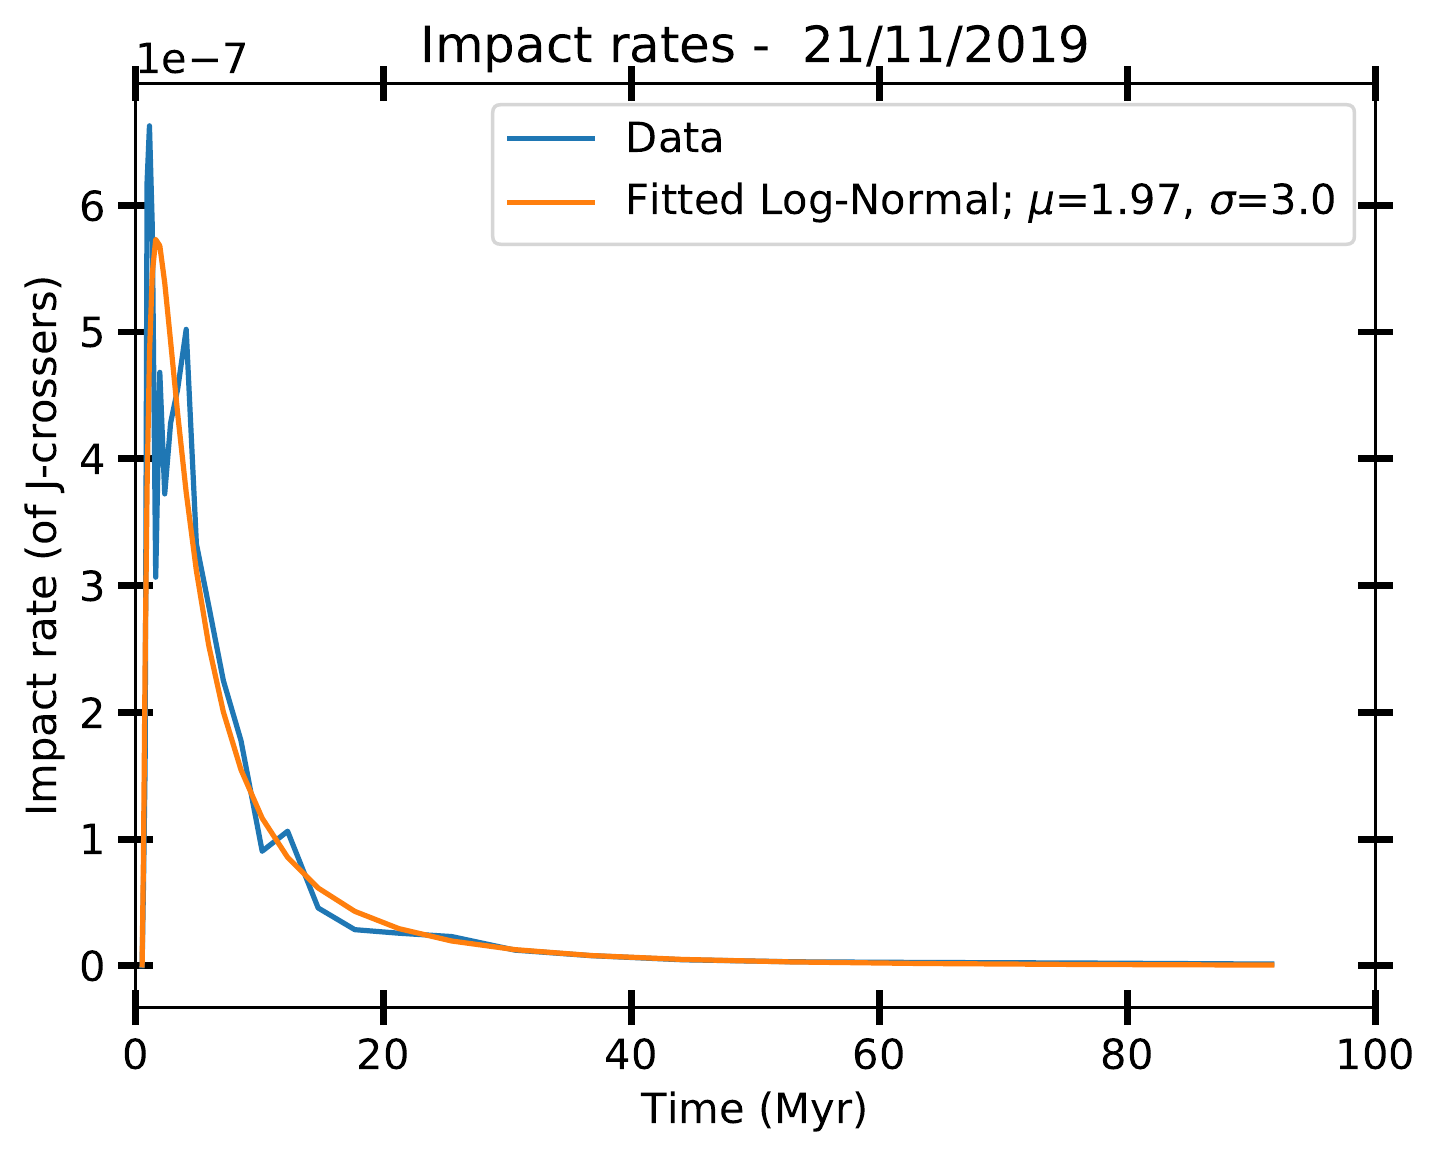}
    \caption{The fraction of jupiter-crossers impacting Earth as a function of time after companion is captured. In blue we show the data and in orange we show a  fitted log-normal function with a mean of 1.97 Myr and standard deviation of 3.0 Myr.}
    \label{fig:my_label}
\end{figure}
\begin{table}
    \centering
    \caption{The fraction of asteroids in the 100 Myr set 1 simulations that have each possible final fate, where: \newline $F_\oplus^\dagger$ - Earth hit, \newline $F_\odot$ - Sun hit, \newline $F_J$ - Jupiter hit, \newline $F_{\rm eject}$ - Ejected, \newline $F_{\rm remain}$ - Remaining.\newline Note: The * denotes outcomes where we have 30 or less asteroids}
    \begin{tabular}{|l| c c c c c|}
    \hline
    System & $F_\oplus^\dagger$ & $F_\odot$ & $F_J$ & $F_{\rm eject}$ & $F_{\rm remain}$ \\
    \hline
ck1.1 & 0.0028 & 0.0527 & 0.0007* & 0.8945 & 0.0493 \\ 
ck1.2 & 0.0026 & 0.0769 & 0.0008* & 0.8775 & 0.0423 \\ 
ck1.3 & 0.0029 & 0.1347 & 0.0009* & 0.8546 & 0.0069 \\ 
ck1.4 & 0.0033 & 0.1746 & 0.0012* & 0.8191 & 0.0021 \\ 
ck1.5 & 0.0025 & 0.1551 & 0.0016* & 0.8392 & 0.0017 \\ 
k1.1 & 0.0006* & 0.0093 & 0.0004* & 0.2256 & 0.7645 \\ 
k1.2 & 0.0008* & 0.0234 & 0.0002* & 0.3846 & 0.5911 \\ 
k1.3 & 0.0024* & 0.1268 & 0.0008* & 0.8062 & 0.0637 \\
f1.1 & 0.0000* & 0.0025 & 0.0000* & 0.0527 & 0.9448 \\ 
f1.2 & 0.0006* & 0.0143 & 0.0004* & 0.2568 & 0.7278 \\ 
f1.3 & 0.0016* & 0.1252 & 0.0011* & 0.7786 & 0.0936 \\ 
f1.4 & 0.0024 & 0.1756 & 0.0008* & 0.8186 & 0.0027 \\ 
f1.5 & 0.0033 & 0.1574 & 0.0012* & 0.8366 & 0.0021 \\
\hline

    \end{tabular}
    \label{tab:final_state}
\end{table}
\begin{table}
\centering
    \begin{tabular}{|l|c c c c|}
    \hline
    System & $f_{\rm Jcross}$ & $f_{\rm Ecross}$ & $f_{\rm E,CE}$ & $f_{\rm Ehit}$ \\
    \hline
ck1.1 & 0.9271 & 0.1284 & 0.2213 & 0.1063 \\ 
ck1.2 & 0.9002 & 0.1678 & 0.1718 & 0.0987 \\ 
ck1.3 & 0.9389 & 0.2449 & 0.1342 & 0.0925 \\ 
ck1.4 & 0.9725 & 0.2974 & 0.1164 & 0.0966 \\ 
ck1.5 & 0.9547 & 0.2866 & 0.1074 & 0.0835 \\ 
k1.1 & 0.1972 & 0.0609 & 0.4251 & 0.1078 \\ 
k1.2 & 0.3004 & 0.0648 & 0.4961 & 0.0881 \\ 
k1.3 & 0.7672 & 0.1132 & 0.3036 & 0.0892 \\ 
f1.1 & 0.0481 & 0.0873 & 0.3452 & 0.0345 \\ 
f1.2 & 0.2326 & 0.1103 & 0.2183 & 0.1071 \\ 
f1.3 & 0.8256 & 0.2177 & 0.1425 & 0.0625 \\ 
f1.4 & 0.9518 & 0.2789 & 0.1302 & 0.0681 \\ 
f1.5 & 0.9301 & 0.2803 & 0.1214 & 0.0932 \\ 
\hline
    \end{tabular}
    \caption{Caption}
    \label{tab:melvyntable}
\end{table}
\textbf{Key}:
\begin{itemize}
    \item $N_{\rm tot}$ -- Total number of asteroids
    \item $f_1$ -- Number of asteroids initial theoretical $r_{\rm min}<10$ divided by $N_{\rm tot}$
    \item $f_2$ -- Number of asteroids getting $r_{\rm min}<10$ in simulation divided by $N_{\rm tot}$
    \item $f_3$ -- Number of asteroid that get within $500R_\oplus$ of E divided by number of asteroids getting within $r_{\rm min}<10$ ($f_2N_{\rm tot}$). 
    \item $f_4$ -- Number of asteroids getting within $100R_\oplus$ divided by number that get within $500R_\oplus$
    \item $F_1$ -- Number of asteroids with $r_{\rm min}>10$  divided by $N_{\rm tot}$
    \item  $F_{1E}$ -- Number of asteroids that are removed with $r_{\rm min}>10$  divided by $N_{\rm tot}$
    \item $F_2$ -- Number of asteroids with $1<r_{\rm min}<10$  divided by $N_{\rm tot}$
    \item $F_{2E}$ -- Number of asteroids that are removed with $1<r_{\rm min}<10$  divided by $N_{\rm tot}$
    \item $F_3$ -- Number of asteroids with $r_{\rm min}<1$  divided by $N_{\rm tot}$
    \item $F_{3E}$ -- Number of asteroids that are removed with $r_{\rm min}<1$  divided by $N_{\rm tot}$
    \item $F_j$ -- Number of asteroids removed by hitting J divided by $N_{\rm tot}$
    \item $F_\oplus$ -- Number of asteroids removed by hitting Earth  divided by $N_{\rm tot}$
    \item $F_\odot$ -- Number of asteroids removed by hitting star divided by $N_{\rm tot}$
    \item $num_1$ -- Number of asteroids initial theoretical $r_{\rm min}<10$ 
    \item $num_2$ -- Number of asteroids getting $r_{\rm min}<10$ in simulation 
    \item $num_3$ -- Number of asteroid that get within $500R_\oplus$ of E
    \item $num_4$ -- Number of asteroids getting within $100R_\oplus$ of E
    \item $NUM_1$ -- Number of asteroids with $r_{\rm min}>10$
    \item $NUM_{1E}$ -- Number of asteroids that are removed with $r_{\rm min}>10$
    \item $NUM_2$ -- Number of asteroids with $1<r_{\rm min}<10$
    \item $NUM_{2E}$ -- Number of asteroids that are removed with $1<r_{\rm min}<10$
    \item $NUM_3$ -- Number of asteroids with $r_{\rm min}<1$
    \item $NUM_{3E}$ -- Number of asteroids that are removed with $r_{\rm min}<1$
    \item $NUM_j$ -- Number of asteroids removed by hitting J
    \item $NUM_\oplus$ -- Number of asteroids removed by hitting Earth 
    \item $NUM_\odot$ -- Number of asteroids removed by hitting star
\end{itemize}
\begin{landscape}

\begin{table}
    \centering
    \begin{tabular}{|c| c c c c | c c | c c| c c | c c c |}
    \hline
    System & $f_1$ & $f_2$ & $f_3$ & $f_4$ & $F_1$ & $F_{1E}$ & $F_2$ & $F_{2E}$ & $F_3$ & $F_{3E}$ & $F_j$ & $F_\oplus$ & $F_\odot$\\
    \hline
    ck1.1 & 1.0 & 0.927 & 0.028 & 0.106 & 0.073 & 0.028 & 0.808 & 0.801 & 0.119 & 0.066 & 0.00075 & 0.0028 & 0.053 \\ 
    ck1.2 & 1.0 & 0.9 & 0.029 & 0.099 & 0.1 & 0.062 & 0.749 & 0.741 & 0.151 & 0.074 & 0.00077 & 0.00256 & 0.077 \\ 
    ck1.3 & 1.0 & 0.939 & 0.033 & 0.092 & 0.061 & 0.057 & 0.709 & 0.703 & 0.23 & 0.094 & 0.00091 & 0.00285 & 0.135  \\ 
    ck1.4 & 1.0 & 0.972 & 0.035 & 0.097 & 0.028 & 0.027 & 0.683 & 0.678 & 0.289 & 0.114 & 0.001 & 0.00325 & 0.175 \\ 
    ck1.5 & 1.0 & 0.955 & 0.031 & 0.083 & 0.045 & 0.045 & 0.681 & 0.677 & 0.274 & 0.117 & 0.002 & 0.0025 & 0.155 \\ 
    \hdashline
    k1.1 & 0.053 & 0.197 & 0.026 & 0.108 & 0.803 & 0.041 & 0.185 & 0.175 & 0.012 & 0.006 & 0.0004 & 0.0006 & 0.009 \\
    k1.2 & 0.14 & 0.3 & 0.032 & 0.088 & 0.7 & 0.112 & 0.281 & 0.263 & 0.019 & 0.009 & 0.0002 & 0.0008 & 0.023 \\ 
    k1.3 & 0.362 & 0.767 & 0.034 & 0.089 & 0.233 & 0.173 & 0.68 & 0.597 & 0.087 & 0.037 & 0.0008 & 0.0024 & 0.127 \\ 
    \hdashline
    f1.1 & 0.012 & 0.048 & 0.03 & 0.034 & 0.952 & 0.008 & 0.044 & 0.043 & 0.004 & 0.002 & 0.0 & 0.0 & 0.002 \\
    f1.2r & 0.004 & 0.014 & 0.018 & 0.0 & 0.986 & 0.003 & 0.014 & 0.013 & 0.001 & 0.0 & 5e-05 & 0.0 & 0.0 \\ 
    f1.2 & 0.09 & 0.233 & 0.024 & 0.107 & 0.767 & 0.042 & 0.207 & 0.201 & 0.026 & 0.012 & 0.0004 & 0.0006 & 0.014 \\
    f1.2r & 0.044 & 0.114 & 0.019 & 0.093 & 0.886 & 0.03 & 0.105 & 0.102 & 0.009 & 0.004 & 0.00015 & 0.0002 & 0.006 \\ 
    f1.3 & 0.336 & 0.826 & 0.031 & 0.062 & 0.174 & 0.088 & 0.646 & 0.623 & 0.18 & 0.068 & 0.001 & 0.0016 & 0.125 \\ 
    f1.3r & 0.139 & 0.469 & 0.031 & 0.076 & 0.531 & 0.08 & 0.376 & 0.355 & 0.093 & 0.031 & 0.0006 & 0.0011 & 0.07 \\ 
    f1.4 & 0.797 & 0.952 & 0.036 & 0.068 & 0.048 & 0.047 & 0.686 & 0.669 & 0.265 & 0.102 & 0.0008 & 0.0024 & 0.176 \\
    f1.4r & 0.333 & 0.849 & 0.036 & 0.064 & 0.151 & 0.108 & 0.625 & 0.597 & 0.225 & 0.077 & 0.00095 & 0.00195 & 0.163 \\ 
    f1.5 & 0.951 & 0.93 & 0.034 & 0.093 & 0.07 & 0.07 & 0.669 & 0.656 & 0.261 & 0.111 & 0.001 & 0.003 & 0.157 \\ 
    \hline
    \end{tabular}
    \label{tab:my_label}
\end{table}
\end{landscape}
\begin{landscape}
\begin{table}
    \centering

    \begin{tabular}{|c| c c c c c| c c | c c| c c | c c c |}
    \hline
    System & $N_{tp}$ & $num_1$ & $num_2$ & $num_3$ & $num_4$ & $NUM_1$ & $NUM_{1E}$ & $NUM_2$ & $NUM_{2E}$ & $NUM_{3}$ & $NUM_{3E}$ & $NUM_\jupiter$ & $NUM_\oplus$ & $NUM_\odot$ \\
    \hline
    ck1.1 & 37.5k & 37.5k &34767 & 988 & 105 & 2733 & 1047 & 30303 & 30036 & 4464 & 2459 & 28 & 105 & 1975 \\ 
    ck1.2 & 37.5k & 37.5k & 33758 & 973 & 96 & 3742 & 2328 & 28095 & 27804 & 5663 & 2776 & 29 & 96 & 2882\\ 
    ck1.3 & 37.5k & 37.5k & 35208 & 1157 & 107 & 2292 & 2143 & 26585 & 26372 & 8623 & 3534 & 34 & 107 & 5052 \\ 
    ck1.4 & 37.5k & 37.5k & 36468 & 1263 & 122 & 1032 & 1026 & 25621 & 25427 & 10847 & 4264 & 37 & 122 & 6546 \\ 
    ck1.5 & 37.5k & 37.5k & 35800 & 1102 & 92 & 1700 & 1698 & 25541 & 25369 & 10259 & 4404 & 60 & 92 & 5812 \\ 
    \hdashline
    k1.1 & 20k & 1061 & 3940 & 102 & 11 & 16060 & 817 & 3700 & 3503 & 240 & 114 & 7 & 11 & 178 \\ 
    k1.2 & 20k & 2795 & 6007 & 193 & 17 & 13993 & 2244 & 5618 & 5267 & 389 & 181 & 4 & 17 & 468 \\ 
    k1.3 & 20k & 7239 & 15340 & 527 & 47 & 4660 & 3456 & 13604 & 11934 & 1736 & 735 & 17 & 47 & 2537 \\ 
    \hdashline
    f1.1 & 20k & 232 & 962 & 29 & 1 & 19038 & 153 & 878 & 858 & 84 & 43 & 0 & 1 & 50 \\ 
    f1.1r & 20k & 85 & 283 & 5 & 0 & 19717 & 66 & 270 & 264 & 13 & 10 & 1 & 0 & 3 \\ 
    f1.2 & 20k & 1791 & 4653 & 112 & 12 & 15347 & 843 & 4140 & 4017 & 513 & 248 & 9 & 12 & 285 \\ 
    f1.2r & 20k & 876 & 2280 & 43 & 4 & 17720 & 609 & 2092 & 2047 & 188 & 86 & 3 & 4 & 115 \\
    f1.3 & 20k & 6727 & 16511 & 512 & 32 & 3489 & 1760 & 12917 & 12454 & 3594 & 1357 & 20 & 32 & 2504 \\ 
    f1.3r & 20k & 2774 & 9384 & 290 & 22 & 10616 & 1609 & 7527 & 7105 & 1857 & 612 & 12 & 22 & 1404 \\ 
    f1.4 & 20k & 15948 & 19037 & 690 & 47 & 963 & 945 & 13728 & 13384 & 5309 & 2042 & 17 & 47 & 3511 \\ 
    f1.4r & 20k & 6651 & 16988 & 612 & 39 & 3012 & 2154 & 12492 & 11947 & 4496 & 1549 & 19 & 39 & 3263 \\ 
    f1.5 & 20k & 19027 & 18599 & 633 & 59 & 1401 & 1395 & 13385 & 13114 & 5214 & 2222 & 20 & 59 & 3148 \\ 
    \hline
    \end{tabular}
    \label{tab:my_label}
\end{table}
\end{landscape}

\clearpage
\begin{table}
    \centering
\caption*{Time limited runs ($10$ Myr)}
    \begin{tabular}{|c| c c | c c c|}
    \hline
    System & $f_1$ & $f_2$ & $K(I_c)$ & $cK(I_c)$ & $cK(I_c)$/$K(I_c)$ \\
    \hline
    k1.1 & 0.05 & 0.06 & 0.22 & 0.01 & 0.05\\
    k1.2 & 0.14 & 0.11 & 0.69 & 0.09 & 0.13\\
    k1.3 & 0.36 & 0.36 & 0.92 & 0.33 & 0.36 \\
    \hdashline
    f1.1 & 0.01 & 0.01 & 0.22 & 0.01 & 0.05\\
    f1.1r & 0.004 & 0.005 & 0.004 & 0.12 & 0.03\\
    f1.2 & 0.09 & 0.08 & 0.69 & 0.09 & 0.13\\
    f1.2r & 0.04 & 0.04 & 0.39 & 0.04 & 0.12\\
    f1.3 & 0.34 & 0.39 & 0.92 & 0.33 & 0.36\\
    f1.3r & 0.14 & 0.12 & 0.74 & 0.14 & 0.19\\
    f1.4 & 0.80 & 0.81 & 0.99 & 0.79 & 0.79\\
    f1.4r & 0.33 & 0.38 &  0.92 & 0.33 & 0.36 \\
    f1.5 & 0.95 & 0.91 & 1.00 & 0.95 & 0.95\\
    \hline
    \end{tabular}
    \label{tab:my_label}
\end{table}
